# Supplementary material for: FFHQ-UV: Normalized Facial UV-Texture Dataset for 3D Face Reconstruction
Source: arXiv:2211.13874 source file (2023-03-24)
Supplement: Supplementary file 2 [file tab-supp_eval_recons.tex]

\begin{table}[!h]
    \caption{More evaluations on 3D face reconstruction.}
    \label{supp:tab:more-eval-recons}
    \small
    \centering
    \setlength{\tabcolsep}{0.45em}{
    \begin{tabular}{l|ccccc}
        \toprule
        Methods & \makecell{$\mathcal{N}_{enc}$}  & \makecell{PCA\\tex basis}  & \makecell{w/o \\editing}    & \makecell{w/o \\multi-view}  & Ours\\
        \midrule
        BS Error & - & - & 8.850 & 4.683 & \textbf{4.322} \\
        \midrule
        Similarity & 0.7832 & 0.7946 & 0.7153 & 0.7980 & \textbf{0.8102} \\
        \midrule
        Exp. Acc. & 73\% & 74\% & 69\% & 78\% & \textbf{82\%} \\
        \bottomrule
    \end{tabular}
    }
\end{table}
