# Supplementary material for: FFHQ-UV: Normalized Facial UV-Texture Dataset for 3D Face Reconstruction
Source: arXiv:2211.13874 source file (2023-03-24)
Supplement: Supplementary file 3 [file tab-supp_id_similarity.tex]

\begin{table}[!h]
    \caption{Average ID similarity score.}
    \small
    \centering
    \setlength{\tabcolsep}{0.60em}{
    \begin{tabular}{l|cccc}
        \toprule
        Methods & \makecell{negative \\samples}  & \makecell{w/o \\multi-view}  & \makecell{naive \\blending}  & Ours\\
        \midrule
        w/ orig. FFHQ & 0.0710 & 0.3723 & 0.4092 & \textbf{0.4262} \\
        \midrule
        w/ frontal pose & 0.0594 & 0.8366 & 0.8481 & \textbf{0.8520} \\
        \bottomrule
    \end{tabular}
    }
    \label{supp:tab:id-similarity}
\end{table}
